# Supplementary material for: Approximation spaces of deep neural networks
Source: arXiv:1905.01208 source file (2020-07-17)
Supplement: Supplementary file 1 [file appendix_inverse.tex]

%!TEX root =  main.tex

\section{Proofs for Inverse estimates}

\begin{lem}\label{lem:BesovNormSawTooth}
Let $j \in \N$ and $f_{j} = \underbrace{g \circ \ldots \circ g}_{j\ \text{times}}$ where \noteRG{details needed}. 
For any $0< p \leq \infty$ and $s>0$
\[
|f|_{B^{s}_{p,\infty}(\Omega)} \geq 2^{-1/p-1} 2^{s(j+2)}.
\]
\todo[inline]{Extend to $0<q \leq \infty$, $s \geq 1$ (seems trivial due to existing embeddings between Besov spaces) and to $d \geq 1$ (using $F_{j}(x) = f_{j}(x_{1})$)}
\end{lem}
